# Supplementary material for: Perceptual Artifacts Localization for Image Synthesis Tasks
Source: arXiv:2310.05590 source file (2023-10-09)
Supplement: Supplementary file 1 [file supp_zoom_inpaint_pipeline.tex]

\begin{figure}[!h]
% \vspace{-5 pt}
    \centering
    %[trim=left bottom right top,
    \includegraphics[trim=0in 1.8in 5.3in 0in, clip,width=0.47\textwidth]{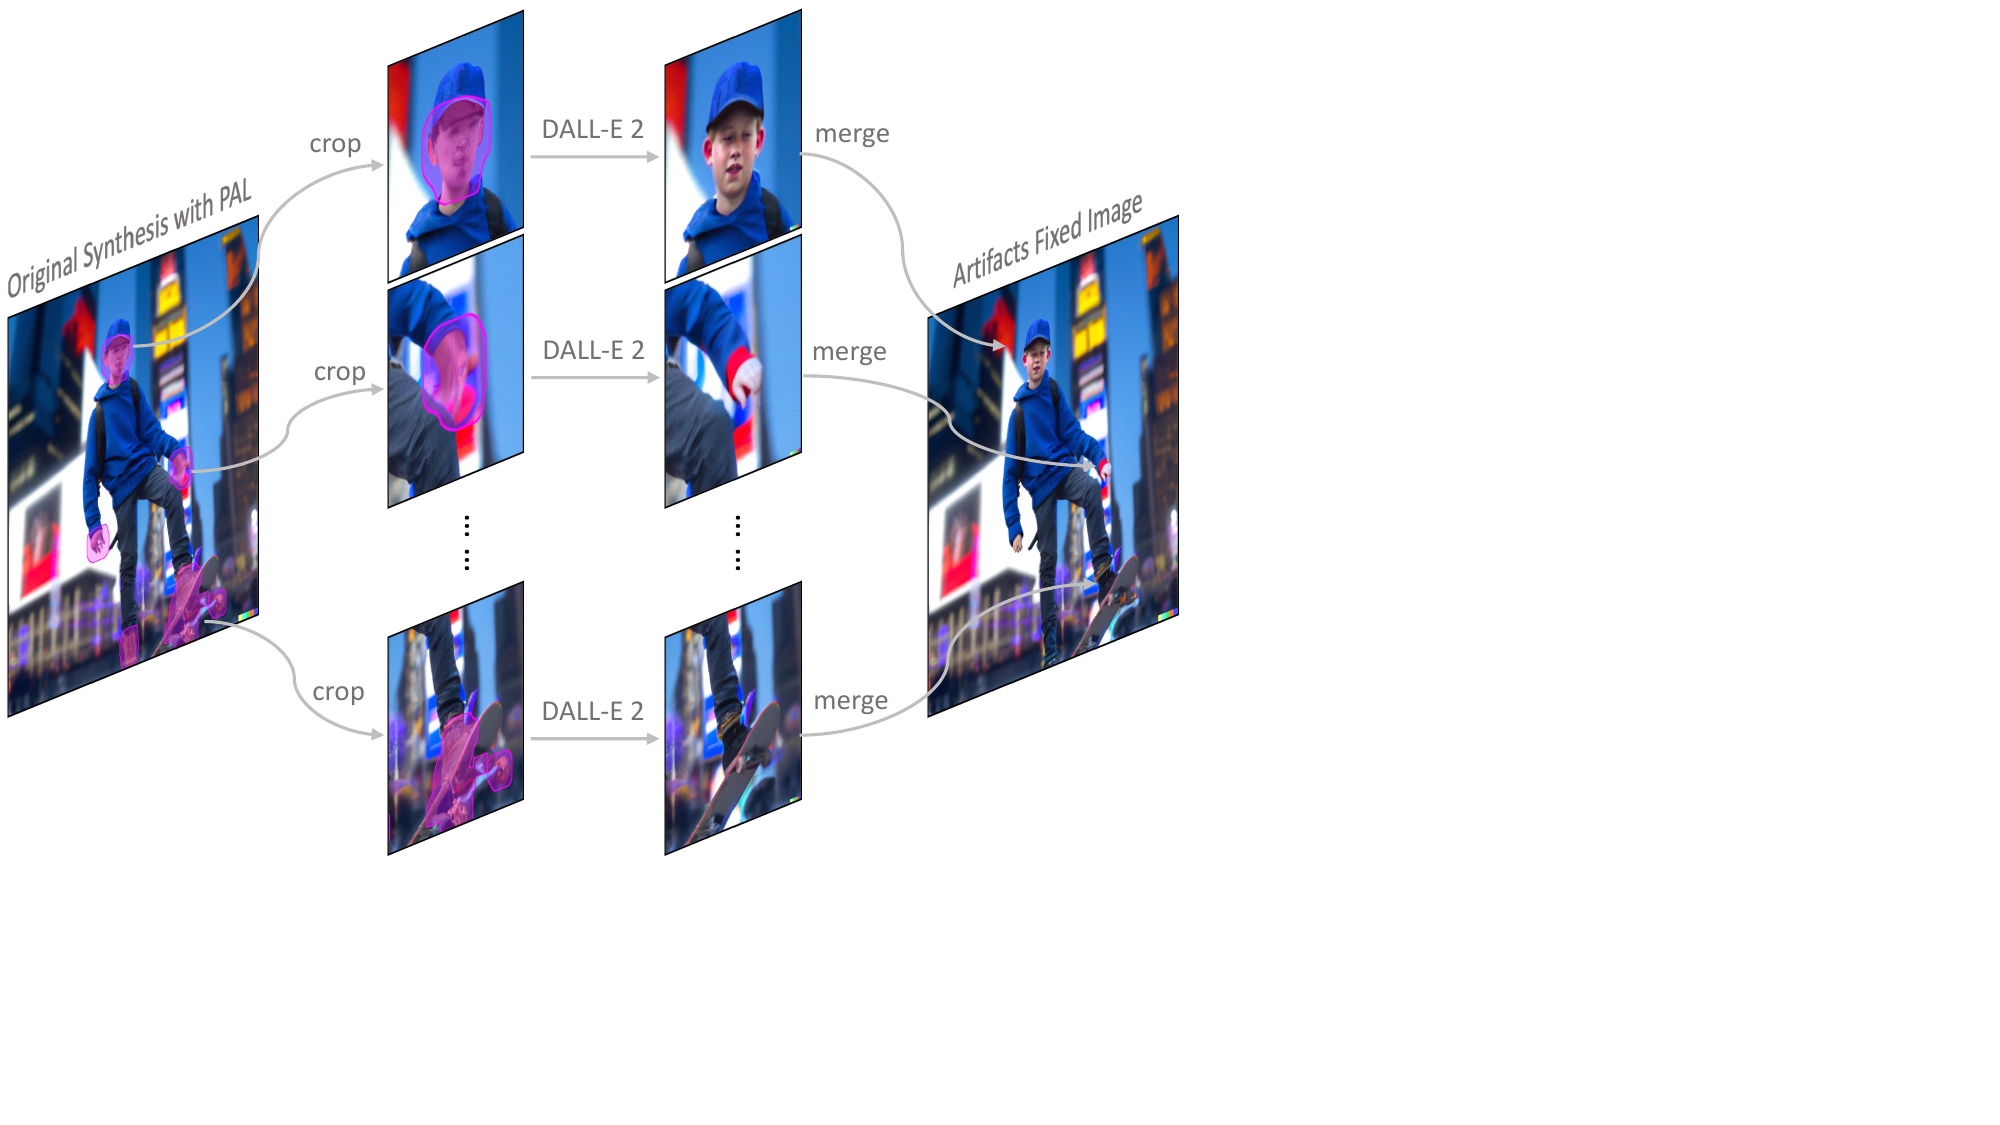}
    % \vspace{-10 pt}
    \caption{A zoom-in inpainting pipeline that can fix perceptual artifacts for object details. In this pipeline, the original generated image is first cropped into multiple patches based on the perceptual artifacts segmentation. Afterwards, each cropped patch is fed into DALL-E 2 inpainting \cite{ramesh2022hierarchical} to fix the perceptual artifacts, and finally merged back into the full image. }
    \label{fig:supp_zoom_inpaint_pipeline}
    \vspace{-10 pt}
\end{figure}
